# Supplementary material for: Contact Forces in Microgel Suspensions
Source: arXiv:2509.25583 ancillary file (2026-09-15)
Supplement: Supplementary file 1 [file Supplementary.pdf]

# Contact Forces in Microgel Suspensions Supplementary Material

Fran Ivan Vrban,<sup>1</sup> Antonio Šiber,<sup>2,3</sup> and Primož Ziherl<sup>1,3</sup>

<sup>1</sup>*Faculty of Mathematics and Physics, University of Ljubljana,  
Jadranska 19, SI-1000 Ljubljana, Slovenia*

<sup>2</sup>*Institute of Physics, Bijenička cesta 46, HR-10000 Zagreb, Croatia*

<sup>3</sup>*Jožef Stefan Institute, Jamova 39, SI-1000 Ljubljana, Slovenia*

(Dated: November 1, 2025)

## I. RESTING DROP

An isolated, resting drop is spherical and pressurized by the surface tension so that its volume  $V_* = 4\pi R_*^3/3$  is smaller than the reference volume  $V_0$ ; here  $R_*$  is the resting radius. The resting volume is obtained by minimizing the liquid-drop free energy

$$F = \frac{V_0}{\chi T} \left( \frac{V}{V_0} - 1 - \ln \frac{V}{V_0} \right) + \gamma_F A_F + \frac{1}{2} \gamma_C A_C \quad (1)$$

for a spherical shape with no contact zones. For this shape, Eq. (1) can be recast as

$$\frac{F}{\gamma_F R_0^2} = 4\pi \left[ \frac{2}{3\Psi} (\lambda_\Psi^3 - 1 - \ln \lambda_\Psi^3) + \lambda_\Psi^2 \right], \quad (2)$$

where  $R_0 = (3V_0/4\pi)^{1/3}$  is the reference radius,

$$\Psi = \frac{2\gamma_F \chi T}{R_0} \quad (3)$$

is the reduced Egelstaff-Widom length, and

$$\lambda_\Psi = \frac{R_*}{R_0} \quad (4)$$

is the ratio of resting and reference radii.

In equilibrium,  $dF/d\lambda_\Psi = 0$  or

$$\lambda_\Psi^3 + \Psi \lambda_\Psi^2 - 1 = 0. \quad (5)$$

This equation can be solved analytically. For  $\Psi < \sqrt[3]{27/4} \approx 1.89$ ,

$$\lambda_\Psi = \frac{1}{3} \left[ -\Psi + \frac{2^{1/3} \Psi^2}{(27 - 2\Psi^3 + 3\sqrt{3}\sqrt{27 - 4\Psi^3})^{1/3}} + \frac{(27 - 2\Psi^3 + 3\sqrt{3}\sqrt{27 - 4\Psi^3})^{1/3}}{2^{1/3}} \right], \quad (6)$$

whereas for  $\Psi > \sqrt[3]{27/4}$

$$\lambda_\Psi = \frac{2\Psi}{3} \cos \left( \frac{1}{3} \arccos \left( \frac{27}{2\Psi^3} - 1 \right) \right) - \frac{\Psi}{3}. \quad (7)$$

In almost incompressible as well as in very compressible drops this result simplifies considerably. If  $\Psi \ll 1$ , we expect that  $\lambda_\Psi$  is just a little smaller than unity. By writing  $\lambda_\Psi = 1 + w$ , expanding Eq. (5) in terms of  $w$ , and solving for  $w$  we find that

$$\lambda_\Psi(\Psi \ll 1) \approx 1 - \frac{\Psi}{3}. \quad (8)$$

On the other hand, if  $\Psi \gg 1$  then  $\lambda_\Psi \ll 1$  and the  $\lambda_\Psi^3$  term in Eq. (5) is small compared to the  $\lambda_\Psi^2$  term. This gives

$$\lambda_\Psi(\Psi \gg 1) \approx \frac{1}{\sqrt{\Psi}}. \quad (9)$$

As shown in Fig. S1a, Eqs. (8) and (9) agree very well with the exact result for  $\Psi \lesssim 0.1$  and  $\Psi \gtrsim 10$ , respectively. By inserting Eqs. (6)-(9) into Eq. (2), we obtain the resting free energy  $F_*$ . The general form of the result is cumbersome but for  $\Psi \ll 1$

$$\frac{F_*(\Psi \ll 1)}{\gamma_F R_0^2} \approx 4\pi \left(1 - \frac{\Psi}{3}\right) \quad (10)$$

whereas for  $\Psi \gg 1$

$$\frac{F_*(\Psi \gg 1)}{\gamma_F R_0^2} \approx \frac{4\pi}{\Psi} \left(\ln \Psi + \frac{1}{3}\right). \quad (11)$$

In Fig. S1b, these two results are plotted against  $\Psi$  together with the exact resting energy.

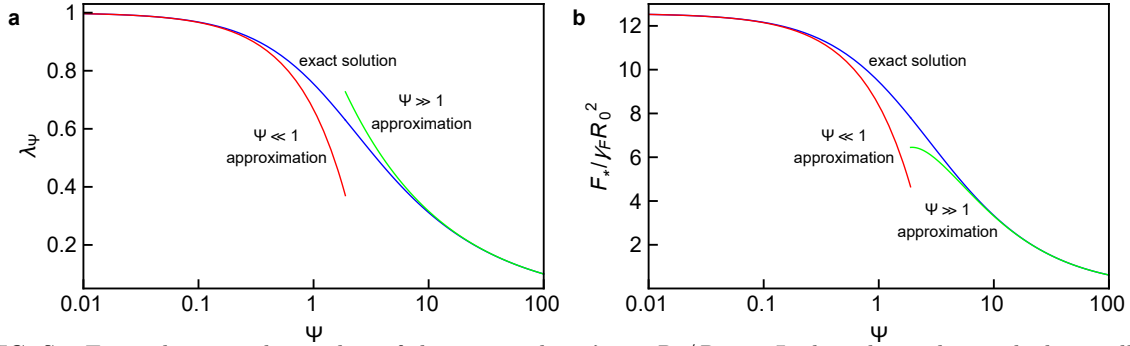

FIG. S1. Exact dimensionless radius of the resting drop  $\lambda_\Psi = R_*/R_0$  vs.  $\Psi$  plotted together with the small- $\Psi$  and large- $\Psi$  approximations [Eqs. (8) and (9)] (a) and the corresponding exact and approximate resting free energies (b).

## II. ENGINEERING AND TRUE INDENTATION

The degree of deformation is best expressed by the dimensionless engineering indentation defined by

$$u = \frac{h}{R_*}. \quad (12)$$

Here  $h$  is the nominal displacement of the center of the contact zone towards the center of the drop upon deformation and  $R_*$  is the resting radius of the undeformed drop. This quantity encodes the degree of deformation based on the undeformed resting state. An alternative approach is to quantify deformation in the deformed final state as sketched in Fig. S2. This may be done in cases where the form of the non-contact domain implies the shape and size of the truncated parts. The simplest (and perhaps the only straightforward) example is a truncated sphere where the radius of the non-contact domain  $R$ , which is generally larger than the resting radius  $R_*$ , uniquely defines the missing spherical caps.

In case of a spherical non-contact domain, Fig. S2 shows that

$$R_* - h = R - \tilde{h}, \quad (13)$$

where  $\tilde{h}$  is the height of the truncated spherical cap. Upon dividing by  $R$  and rearranging, we find that dimensionless true indentation defined by  $\tilde{u} = \tilde{h}/R$  reads

$$\tilde{u} = 1 - \frac{R - \tilde{h}}{R_*} = 1 - \frac{1 - u}{\lambda} = \frac{u}{\lambda} + \frac{\lambda - 1}{\lambda}. \quad (14)$$

Here

$$\lambda = \frac{R}{R_*} \quad (15)$$

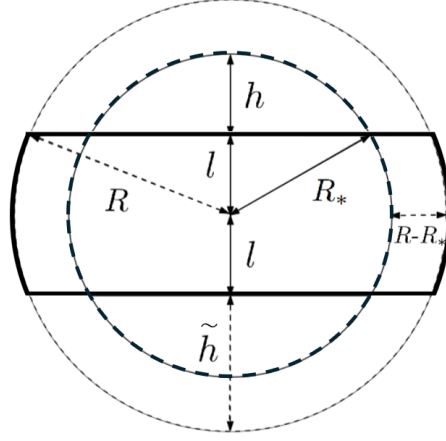

FIG. S2. Engineering indentation  $h$  and true indentation  $\tilde{h}$ : The former is defined as the displacement of the center of the contact zone toward drop center, whereas the latter corresponds to the height of the spherical cap removed from the sphere defined by the non-contact domain so as to create the contact zone.

is the ratio of the radii of the deformed and the resting drop. For small indentations where  $\lambda \approx 1$ , the two radii are not very different so that  $\tilde{u} \approx u$ .

As implied by the insets in Fig. 2a of the main text, the shape of a deformed drop is generally quite different from the truncated sphere, and hence the true indentation cannot be defined unambiguously. Thus we rely on the engineering indentation as the measure of deformation.

### III. EXACT EQUILIBRIUM DROP SHAPES

In Fig. S3, we show a few examples of the the equilibrium drop shapes in the simple cubic (SC) lattice obtained numerically using the Surface Evolver package [1].

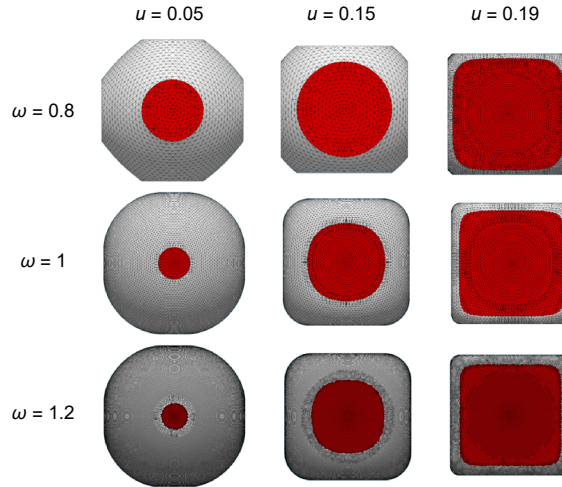

FIG. S3. Select exact equilibrium shapes of  $\Psi = 10^{-3}$  drops in the SC lattice at  $\omega = 0.8, 1$ , and  $1.2$  and  $u = 0.05, 0.15$ , and  $0.19$ . Drawn in black are the edges of the triangulated drop surfaces; hence the darker appearance of the more finely subdivided drops.

#### IV. TRUNCATED SPHERE

This variational shape is an intersection of a sphere and several half-spaces corresponding to a contacts with neighboring drops (Fig. S4a). Each plane that defines a half-space cuts off a spherical cap. Based on relative cap size, we can distinguish between three faceting regimes: In the partial faceting regime, the caps do not intersect whereas in the advanced faceting regime they do, and in the complete faceting regime the non-contact domain no longer exists.

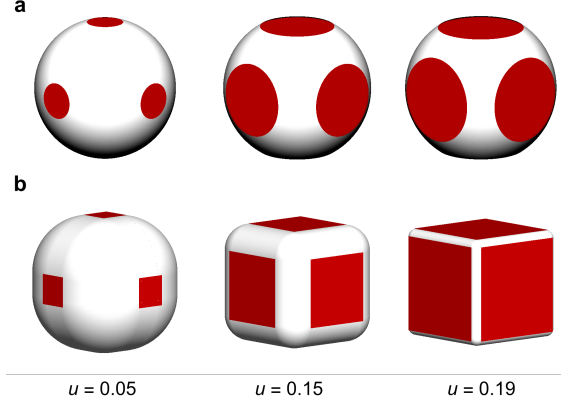

FIG. S4. Sequences of truncated-sphere for  $\Psi = 10$ ,  $\omega = 1$  (a) and non-truncated spheropolyhedral shapes  $\Psi = 10^{-3}$ ,  $\omega = 1.2$  (b) in the simple cubic (SC) lattice for  $u = 0.05, 0.10$ , and  $0.19$ ; the values of  $\Psi$  and  $\omega$  are chosen so as to best emphasize the differences between the two variational shapes at these three indentations. The contact zones are colored red whereas the non-contact domain is white.

The only parameter of the truncated sphere is the ratio of the radius of the non-contact domain and the resting radius

$$\lambda = \frac{R}{R_*}. \quad (16)$$

This ratio depends on  $\Psi$ ,  $\omega$ , and all dimensionless engineering indentations  $u_i$ . The equilibrium value of  $\lambda$  is determined by minimizing the free energy in Eq. (1); in incompressible drops,  $\lambda$  is computed by minimizing the surface energy in Eq. (1) at constant volume.

##### A. Drop volume and area

Here we consider drops arranged in so-called regular lattices where the distances of a site to all nearest neighbors and thus the indentations  $u_i$  are the same; these lattices are face-centered cubic (FCC), simple cubic (SC), and diamond cubic (DC) lattice with the coordination numbers  $z = 12, 6$ , and  $4$ <sup>1</sup>, respectively. We are interested primarily in small deformations, i.e., in the partial faceting regime where the contact zones are circles. The three geometric quantities needed to calculate the deformation free energy are the volume of a spherical cap corresponding to a contact zone, the cap area, and the cap base area. The cap volume reads

$$V_{\text{cap}} = \pi \tilde{h}^2 \left( R - \frac{\tilde{h}}{3} \right) = \frac{\pi R_*^3}{3} (\lambda - 1 + u)^2 (2\lambda + 1 - u), \quad (17)$$

[where  $\lambda = R/R_*$  and  $u = h/R_* = \lambda(\tilde{h}/R - 1) + 1$  as explained in Sec. II] so that the volume of a drop of radius  $R = \lambda R_*$  with  $z$  neighbors is

$$V = \frac{4\pi R^3}{3} - z V_{\text{cap}} = \frac{4\pi R_*^3}{3} \left[ \lambda^3 - \frac{z}{4} (\lambda - 1 + u)^2 (2\lambda + 1 - u) \right]. \quad (18)$$

<sup>1</sup> At indentations  $u \gtrsim 0.36$ , each drop in the DC lattice also pushes against 12 next-nearest neighbors so that the coordination number is no longer  $z = 4$ .

The cap area is given by

$$A_{\text{cap}} = 2\pi R\tilde{h} = 2\pi R_*^2\lambda(\lambda - 1 + u) \quad (19)$$

and thus the area of the non-contact domain reads

$$A_F = 4\pi R^2 - zA_{\text{cap}} = 2\pi R_*^2[2\lambda^2 - z\lambda(\lambda - 1 + u)]. \quad (20)$$

The cap base area is  $A_{\text{base}} = \pi\tilde{h}(2R - \tilde{h}) = \pi R_*^2(\lambda^2 - 1 + 2u - u^2)$  and the combined area of the contact zones is

$$A_C = zA_{\text{base}} = z\pi R_*^2(\lambda^2 - 1 + 2u - u^2). \quad (21)$$

Here we used Eq. (13) to express  $V_{\text{cap}}$ ,  $A_{\text{cap}}$ , and  $A_{\text{base}}$  in terms of the reduced engineering indentation  $u$ . In the partial faceting regime, these three quantities do not depend on the exact location of the contact zones as long as their indentations and therefore areas are the same.

## B. Constraints

All geometric quantities pertaining to the drop— $A_{\text{cap}}$ ,  $A_{\text{base}}$ ,  $A_F$ ,  $V_{\text{cap}}$ , and  $V$ —must be positive. The condition that  $A_{\text{cap}} > 0$  implies that

$$\lambda > 1 - u; \quad (22)$$

$A_{\text{base}} > 0$  leads to the same inequality as both  $A_{\text{cap}} > 0$  and  $A_{\text{base}} > 0$  rely on  $\tilde{h} > 0$ . On the other hand,  $A_F > 0$  means that  $\lambda < z(1 - u)/(z - 2)$  but in the SC lattice this condition is less restrictive than that pertaining to the validity of the partial faceting regime as described below by Eq. (24). The condition that  $V_{\text{cap}} > 0$  implies that  $\lambda > -1/2 + u/2$  which is not restrictive because  $u$  cannot exceed 1 and  $\lambda$  must be larger than 0. Also automatically satisfied is the constraint  $V > 0$  which translates into  $\lambda^3 - z(\lambda - 1 + u)^2(2\lambda + 1 - u)/4 > 0$  because it is less restrictive than the condition in Eq. (24).

The geometry of the truncated-sphere shape in the advanced faceting regime where some or all contact zones are truncated circles is more involved, and analytical expressions for volume, area of contact zones, and area of the non-contact domain are far less transparent. In the complete faceting regime, these three quantities simplify because (i) the non-contact domain vanishes and because (ii) the shape of the drop becomes polyhedral and does not depend on indentation so that the ratio  $V/A^{3/2}$  is constant.

In the truncated-sphere approximation, the indentations marking the end of the partial and onset of the complete faceting regime are defined unambiguously. For example, in the SC lattice they correspond to indentations where the radius of the non-contact domain coincides with half of the face and half of the body diagonal of the unit cell, respectively. Since the side of the unit cell

$$a = 2(R_* - h) = 2R_*(1 - u), \quad (23)$$

in the partial faceting regime

$$\lambda(u) < \sqrt{2}(1 - u). \quad (24)$$

whereas in the complete faceting regime

$$\lambda(u) > \sqrt{3}(1 - u). \quad (25)$$

In between these two lies the advanced faceting regime.

## C. Deformation free energy

Using the above results, we can calculate the deformation energy of the truncated sphere shapes. This can be done in the small-tension regime at  $\Psi \ll 1$  where the drop volume is constant and in the large-tension regime at  $\Psi \gg 1$ .

For  $\Psi \ll 1$ , we assume that the bulk energy vanishes and that the deformation free energy consist solely of the surface energy so that

$$\begin{aligned}\Delta F &= \Delta F_{\text{surf}} = \gamma_F A_F + \frac{1}{2} \gamma_C A_C - 4\pi \gamma_F R_*^2 \\ &= \gamma_F 2\pi R_*^2 \left[ 2\lambda^2 - z\lambda(\lambda - 1 + u) \right] + \frac{1}{2} \gamma_C z\pi R_*^2 (\lambda^2 - 1 + 2u - u^2) - 4\pi \gamma_F R_*^2 \\ &= \gamma_F R_0^2 \times 2\pi \lambda_\Psi^2 \left\{ 2(\lambda^2 - 1) + z \left[ -\lambda(\lambda - 1 + u) + \frac{\omega}{2} (\lambda^2 - 1 + 2u - u^2) \right] \right\}.\end{aligned}\quad (26)$$

where we used Eqs. (19)-(21). The volume constraint reduces to

$$\lambda^3 - \frac{z}{4} (\lambda - 1 + u)^2 (2\lambda + 1 - u) = 1, \quad (27)$$

where we used Eq. (18); this equation must be solved for  $\lambda$ . Exact solution exists but is quite cumbersome; at  $u \ll 1$ , a reasonable approximation valid wherever  $\lambda$  is just a little larger than unity is

$$\lambda \approx 1 + \frac{zu^2}{4}. \quad (28)$$

This approximation gives the deformation energy per contact zone that reads

$$\frac{\Delta F}{z\gamma_F R_0^2} \approx 2\pi \left( 1 - \frac{2\Psi}{3} \right) \left\{ (\omega - 1)u + \left[ 1 - \frac{\omega}{2} + \frac{z(\omega - 1)}{4} \right] u^2 \right\}. \quad (29)$$

Here we retained terms up to second order in  $u$  and we inserted  $\lambda_\Psi \approx 1 - \Psi/3$ .

The validity of Eq. (29) is evidently limited; for example, it fails to reproduce the bound state at  $u = 0$  and  $\omega < 0$  (seen in Fig. 2a of the main text) and it predicts that to lowest order,  $\Delta F \propto u$  for  $\omega \neq 1$ , which is incorrect. On the other hand, Eq. (29) shows that (i) the small- $u$   $\Delta F$  is attractive for  $\omega < 1$  and repulsive for  $\omega > 1$  and that (ii) at  $\Psi \ll 1$  the deformation free energy is not pairwise additive because the energy per contact depends on the number of contacts, which is conceptually consistent with Fig. 4 of the main text (although this dependence vanishes as  $\omega = 1$ ).

For  $\Psi \gg 1$ , we start by calculating the volume change relative to the resting volume  $V_*$ :

$$\Delta V = V - V_* = \frac{4\pi R_*^3}{3} \left[ \lambda^3 - 1 - \frac{z}{4} (\lambda - 1 + u)^2 (2\lambda + 1 - u) \right]. \quad (30)$$

where  $V$  is given by Eq. (18). If indentations are small compared to  $R_*$ ,  $\Delta V \ll V_*$  and the bulk term of the deformation energy is

$$\Delta F_{\text{bulk}} = \chi_T^{-1} \left[ \Delta V - V_0 \ln \left( 1 + \frac{\Delta V}{V_*} \right) \right] \approx -\chi_T^{-1} V_0 \left[ \frac{\Delta V}{V_*} - \frac{1}{2} \left( \frac{\Delta V}{V_*} \right)^2 \right], \quad (31)$$

where we expanded the logarithm and then neglected  $\Delta V/V_0 = \Delta V/V_* \times V_*/V_0 = \Delta V/V_* \times \lambda_\Psi^3$  because for  $\Psi \gg 1$ ,  $\lambda_\Psi \approx 1/\sqrt{\Psi}$  [Eq. (8)] is small compared to unity. The ratio

$$\frac{\Delta V}{V_*} = \lambda^3 - 1 - \frac{z}{4} (\lambda - 1 + u)^2 (2\lambda + 1 - u) \quad (32)$$

so that

$$\begin{aligned}\frac{\Delta F_{\text{bulk}}}{z\gamma_F R_0^2} &= -\frac{8\pi}{3\Psi z} \left[ \lambda^3 - 1 - \frac{z}{4} (\lambda - 1 + u)^2 (2\lambda + 1 - u) \right] \\ &\times \left\{ 1 - \frac{1}{2} \left[ \lambda^3 - 1 - \frac{z}{4} (\lambda - 1 + u)^2 (2\lambda + 1 - u) \right] \right\}.\end{aligned}\quad (33)$$

The surface term reads

$$\Delta F_{\text{surf}} = \gamma_F \Delta A_F + \gamma_F \omega \Delta A_C, \quad (34)$$

where  $\Delta A_F$  and  $\Delta A_C$  are the relative changes of the area of the non-contact domain and the contact-zone area, respectively, that arise upon indentation. The change of the area of the non-contact domain

$$\Delta A_F = A_F - 4\pi R_*^2, \quad (35)$$

where  $A_F$  is given by Eq. (20), whereas the change of area of the contact zones is evidently

$$\Delta A_C = A_C \quad (36)$$

where  $A_C$  is given by Eq. (21). After inserting  $\lambda_\Psi \approx 1/\sqrt{\Psi}$  for  $\Psi \gg 1$  [Eq. (9)], we obtain

$$\frac{\Delta F_{\text{surf}}}{z\gamma_F R_0^2} = \frac{2\pi}{\Psi} \left[ \frac{2(\lambda^2 - 1)}{z} - \lambda(\lambda - 1) - \lambda u + \omega \left( \frac{\lambda^2 - 1}{2} + u - \frac{u^2}{2} \right) \right]. \quad (37)$$

If we assume that  $\lambda = 1$  then

$$\begin{aligned} \frac{\Delta F_{\text{bulk}}}{z\gamma_F R_0^2} &= -\frac{8\pi}{3\Psi z} \left[ -\frac{z}{4} u^2 (3 - u) \right] \left\{ 1 - \frac{1}{2} \left[ -\frac{z}{4} u^2 (3 - u) \right] \right\} \\ &= \frac{2\pi}{3\Psi} u^2 (3 - u) \left[ 1 + \frac{z}{8} u^2 (3 - u) \right] \\ &\approx \frac{2\pi}{\Psi} u^2 \left( 1 - \frac{u}{3} \right) \end{aligned} \quad (38)$$

and

$$\frac{\Delta F_{\text{surf}}}{z\gamma_F R_0^2} = \frac{2\pi}{\Psi} \left[ -u + \omega \left( u - \frac{u^2}{2} \right) \right] = \frac{2\pi}{\Psi} \left[ (\omega - 1)u - \frac{\omega}{2} u^2 \right]. \quad (39)$$

These two terms combined give

$$\frac{\Delta F}{z\gamma_F R_0^2} = \frac{2\pi}{\Psi} \left[ (\omega - 1)u + \left( 1 - \frac{\omega}{2} \right) u^2 \right]. \quad (40)$$

This is Eq. (4) from Ref. [2].

#### D. Pairwise additivity in large-tension regime

The truncated sphere shapes can be used to show that at large tensions the drop-drop interaction is pairwise additive. We begin by calculating the bulk term equal to the work done against the pressure within the drop. This pressure depends on the drop volume, which makes the deformation free energy non-pairwise-additive. However, at  $\Psi \gg 1$  the increase of pressure due to indentation is small compared to the reference pressure as shown below, and thus the pressure in a deformed drop is not very different from the reference pressure. As a result, the bulk deformation free energy is pairwise additive.

Specifically,

$$p(V) = \frac{1}{\chi T} \left( \frac{V_0}{V} - 1 \right) \quad (41)$$

so that the resting pressure reads

$$p_* = \frac{1}{\chi T} \left( \frac{V_0}{V_*} - 1 \right) = \frac{1}{\chi T} (\lambda_\Psi^{-3} - 1). \quad (42)$$

The increase of pressure due to indentation can be estimated by

$$\Delta p = \left( \frac{\partial p}{\partial V} \right)_{V=V_*} \Delta V, \quad (43)$$

where

$$\left(\frac{\partial p}{\partial V}\right)_{V=V_*} = -\frac{V_0}{\chi_T V^2}\bigg|_{V=V_*} = -\frac{V_0}{\chi_T V_*^2} = -\frac{1}{\chi_T V_0} \left(\frac{V_0}{V_*}\right)^2 = -\frac{1}{\chi_T V_0 \lambda_\Psi^6}. \quad (44)$$

The total volume of the  $z$  indentations is

$$\Delta V = -z \times \pi R_* h^2 = -\pi z R_0^3 \lambda_\Psi^3 u^2 \quad (45)$$

so that

$$\Delta p = \frac{\pi z R_0^3 \lambda_\Psi^3 u^2}{\chi_T V_0 \lambda_\Psi^6} = \frac{3zu^2}{4\chi_T \lambda_\Psi^3} \quad (46)$$

and

$$\frac{\Delta p}{p_*} = \frac{3zu^2}{4(1 - \lambda_\Psi^3)}. \quad (47)$$

If  $\Psi \gg 1$ , then  $\lambda_\Psi \approx 1/\sqrt{\Psi} \ll 1$  and

$$\frac{\Delta p}{p_*} \approx \frac{3zu^2}{4}, \quad (48)$$

which is small.

Equation (48) demonstrates that the pressure within the drop is dominated by the resting pressure. This also shows in the work against it. Since  $p = p_* + (\partial p / \partial V)|_{V=V_*}(V - V_*)$ ,

$$\begin{aligned} W &= -\int_{V_*}^{V_*+\Delta V} p dV = -p_* \Delta V - \left(\frac{\partial p}{\partial V}\right)_{V=V_*} \frac{(\Delta V)^2}{2} \\ &= -p_* \Delta V \left(1 + \frac{\Delta p}{2p_*}\right) = \frac{1}{\chi_T} (\lambda_\Psi^{-3} - 1) \pi z R_0^3 \lambda_\Psi^3 u^2 \left(1 + \frac{3zu^2}{8}\right) \\ &\approx \frac{\pi R_0^3}{\chi_T} z u^2 = z \gamma_F R_0^2 \times 2\pi \frac{R_0}{2\gamma_F \chi_T} u^2 = z \gamma_F R_0^2 \times \frac{2\pi}{\Psi} u^2, \end{aligned} \quad (49)$$

where we approximated  $1 - \lambda_\Psi^3$  by unity because  $\lambda_\Psi \ll 1$  and we neglected the  $u^4$  term. Thus

$$\frac{\Delta F_{\text{bulk}}}{z \gamma_F R_0^2} = \frac{2\pi}{\Psi} u^2 \quad (50)$$

so that the bulk term of the deformation free energy is pairwise additive at large  $\Psi$ . The pairwise-additive nature of the surface term at  $\Psi \gg 1$  is demonstrated in Sec. IIIC.

### E. Receding drop

The truncated sphere shape also admits the receding-drop mode where the contact zones are point-like and their area vanishes. The shape of the receding drop is spherical such that the Laplace pressure condition is satisfied, and the radius of the drop relative to the resting radius  $\lambda = R/R_*$  is a simple function of indentation:

$$\lambda = 1 - u. \quad (51)$$

The deformation free energy reads

$$\begin{aligned} \frac{\Delta F}{z \gamma_F R_0^2} &= \frac{4\pi}{z} \left\{ \frac{2}{3\Psi} [(\lambda^3 - 1)\lambda_\Psi^3 - \ln \lambda^3] + (\lambda^2 - 1)\lambda_\Psi^2 \right\} \\ &= \frac{8\pi}{z} \left\{ \frac{1}{\Psi} \left[ -u \left( 1 - u + \frac{u^2}{3} \right) \lambda_\Psi^3 - \ln(1 - u) \right] - u \left( 1 - \frac{u}{2} \right) \lambda_\Psi^2 \right\}. \end{aligned} \quad (52)$$



Upon expanding the logarithm, we find that the linear term in  $u$  vanishes because of Eq. (5) and that

$$\frac{\Delta F}{z\gamma_F R_0^2} = \frac{8\pi}{z} \left[ \left( \frac{\lambda_\Psi^3 + 1/2}{\Psi} + \frac{\lambda_\Psi^2}{2} \right) u^2 + \frac{1 - \lambda_\Psi^3}{3\Psi} u^3 + \Psi^{-1} \sum_{i=4}^{\infty} \frac{u^i}{i} \right]. \quad (53)$$

The receding-drop mode is relevant at large  $\Psi$  where the drop can be compressed. At  $\Psi \gg 1$  where  $\lambda_\Psi \approx 1/\sqrt{\Psi}$ , we have

$$\frac{\Delta F}{z\gamma_F R_0^2} \approx \frac{8\pi}{z\Psi} \left( u^2 + \sum_{i=3}^{\infty} \frac{u^i}{i} \right). \quad (54)$$

Figure S5 shows the full receding-drop deformation free energy [Eq. (52)] and the leading-order term of the approximation in Eq. (54) for  $\Psi = 1, 10$ , and  $10^2$ .

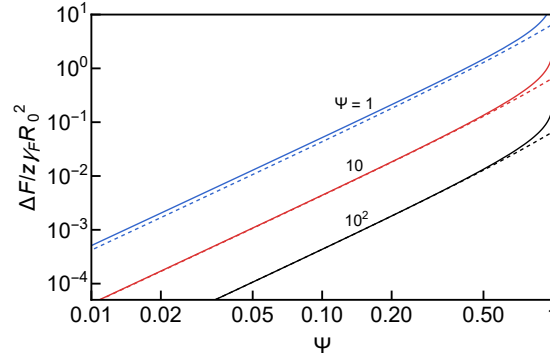

FIG. S5. Energy of the receding drop shape vs. indentation for  $\Psi = 1, 10$ , and  $100$ . solid lines represent the exact result [Eq. (52)] whereas dashed lines show the leading-order term of the  $\Psi \gg 1$  approximation [Eq. (54)], which is proportional to  $u^2$ .

## V. TRUNCATED SUPERBALL

The superball compatible with the symmetry of the simple cubic (SC) lattice is defined by

$$R^m = |x|^m + |y|^m + |z|^m, \quad (55)$$

where  $R$  is half of the pole-to-pole distance and  $m$  is the shape parameter. For  $m = 1$ , the shape reduces to an octahedron, for  $m = 2$  it is a sphere, and for  $m \rightarrow \infty$  it is a cube. In the deformed state, drop shape deviates from the sphere because of the flat contact zones and the concomitant non-spherical form of the non-contact domain. However, at small deformations these two effects are small and hence we can consider a truncated superball at  $m \approx 2$  rather than at an arbitrary  $m$ . Below we derive approximate analytical formulas for the five geometrical quantities of interest: Volume  $V$ , area  $A$ , cap volume  $V_{\text{cap}}$ , cap area  $A_{\text{cap}}$ , and cap base area  $A_{\text{base}}$ .

The superball volume can be calculated exactly and reads

$$V_{\text{SB}} = 8 \frac{[\Gamma(1 + 1/m)]^3}{\Gamma(1 + 3/m)} R^3. \quad (56)$$

To third order in  $a = m - 2$ ,

$$V_{\text{SB}}(R, a) \approx \frac{4\pi R^3}{3} (1 + k_{V1}a + k_{V2}a^2 + k_{V3}a^3), \quad (57)$$

where

$$k_{V1} = \frac{1}{2}, \quad k_{V2} \approx -0.175275 \quad \text{and} \quad k_{V3} \approx 0.0358379. \quad (58)$$

The closed-form expressions for these coefficients exist but are not very illuminating. Reference [3] suggests that there exists no closed-form expression for superball area  $A(R, m)$ . Numerical results based on Eq. (B17) in Ref. [4] show that to third order in  $a$

$$A_{\text{SB}}(R, a) \approx 4\pi R^2 (1 + k_{A1}a + k_{A2}a^2 + k_{A3}a^3), \quad (59)$$

where

$$k_{A1} = \frac{1}{3}, \quad k_{A2} \approx -0.102296, \quad \text{and} \quad k_{A3} \approx 0.0225688. \quad (60)$$

The argument justifying the exact coefficient of the linear term is as follows: The ratio of the coefficients in front of  $a$  in Eqs. (57) and (59) should be  $3/2$  because this ensures that the reduced volume of the superball defined by  $v = 6\sqrt{\pi}V/A^{3/2}$  reads

$$v \approx \frac{1 + a/2}{(1 + a/3)^{3/2}} = 1 + \mathcal{O}(a^2) \quad (61)$$

and is maximal at  $a = 0$ , that is in a sphere. This is guaranteed if the linear terms in  $a$  in the numerator and in the denominator of  $v$  cancel, which implies that the linear-term coefficient in Eq. (59) is  $1/3$ . This reasoning is consistent with the numerically computed superball area for  $|a| \leq 0.5$ ; the second- and third-order coefficients are found by fitting the latter.

The other three quantities are bracketed by their values in the octahedron ( $m = 1$ ), the sphere ( $m = 2$ ), and the cube ( $m \rightarrow \infty$ ). Specifically, in the octahedron

$$V_{\text{cap}} = \frac{2}{3}\tilde{h}^3, \quad (62)$$

$$A_{\text{base}} = 2\tilde{h}^2, \quad (63)$$

and

$$A_{\text{cap}} = 2\sqrt{3}\tilde{h}^2; \quad (64)$$

in the sphere

$$V_{\text{cap}} = \pi\tilde{h}^2(R - \tilde{h}/3), \quad (65)$$

$$A_{\text{base}} = 2\pi\tilde{h}(R - \tilde{h}/2), \quad (66)$$

and

$$A_{\text{cap}} = 2\pi R\tilde{h}; \quad (67)$$

and in the cube,

$$V_{\text{cap}} = 4R^2\tilde{h} \quad (68)$$

$$A_{\text{base}} = 4R^2. \quad (69)$$

and

$$A_{\text{cap}} = 4R^2 + 8R\tilde{h}. \quad (70)$$

In all of these expressions,  $\tilde{h}$  is cap height.

For small  $\tilde{h}$ ,  $V_{\text{cap}}$ ,  $A_{\text{cap}}$ , and  $A_{\text{base}}$  can be calculated by approximating Eq. (55) around  $x \ll R, y \ll R$ , and  $z \approx R$  by a Monge representation

$$z(x, y) \approx R \left\{ 1 - \frac{1}{m} \left[ \left( \frac{x}{R} \right)^m + \left( \frac{y}{R} \right)^m \right] \right\}. \quad (71)$$

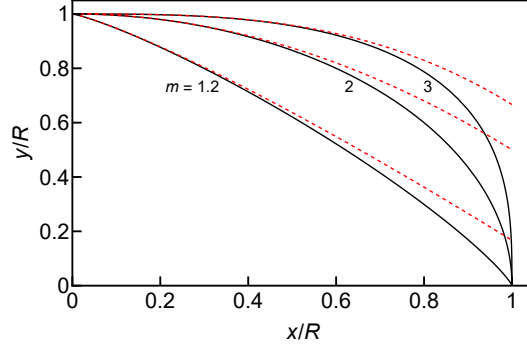

FIG. S6. Profile of the  $m = 1.2, 2$ , and  $3$  superballs in the  $xy$  plane: Solid lines show the exact contour whereas red dashed lines are the corresponding Monge representations valid close to the pole at  $x = 0$  [Eq. (71)].

In Fig. S6, the profiles of the  $m = 1.2, 2$ , and  $3$  superballs in the  $xz$  plane given by Eq. (71) is compared to the exact ones.

Using Eq. (71), we find that

$$V_{\text{cap}} \approx 2\sqrt{\pi} \left(\frac{m}{2}\right)^{2/m} \frac{\Gamma(1+1/m)}{\Gamma(3/2+1/m)} R^3 \left(\frac{\tilde{h}}{R}\right)^{1+2/m}. \quad (72)$$

This reduces to Eq. (62), the quadratic part of Eq. (65), and Eq. (68) for  $m = 1, 2$ , and  $\infty$ , respectively. The comparison of the exact numerical results and Eq. (72) is shown in Fig. S7, where we see that the latter overestimates the cap volume at all  $m$  but that the difference drops to 0 as  $m$  approaches both 1 and  $\infty$ .

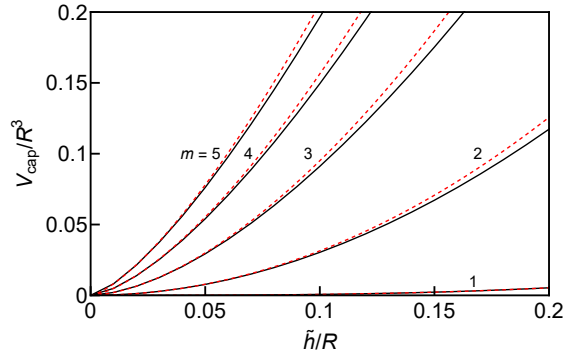

FIG. S7. Exact numerically obtained superball cap volume vs.  $\tilde{h}/R$  for  $m = 1, 1.5, 2, 2.5, 3, 4$ , and  $5$  (black curves). Dashed red curves are obtained using the Monge representation [Eq. (72)].

In a similar manner, we find that

$$A_{\text{base}} \approx 4\sqrt{\pi} \left(\frac{m}{2}\right)^{2/m} \frac{\Gamma(1+1/m)}{\Gamma(1/2+1/m)} R^2 \left(\frac{\tilde{h}}{R}\right)^{2/m}, \quad (73)$$

which reduces to Eq. (63), the linear part of Eq. (66) and Eq. (69) for  $m = 1, 2$ , and  $\infty$ , respectively. In Fig. S8, we compare exact numerical results and Eq. (73) for various  $m$ .

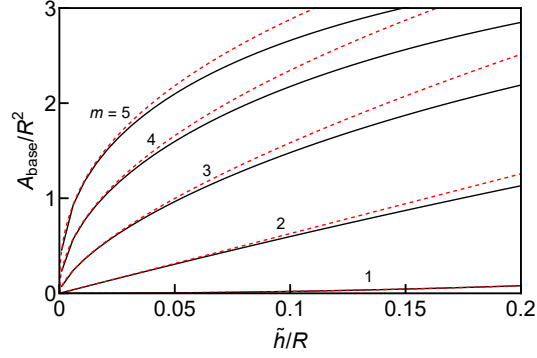

FIG. S8. Exact superball cap base area vs.  $\tilde{h}/R$  for  $m = 1, 2, 3, 4$  and  $5$  (black curves). Dashed red curves show the approximation obtained using the Monge representation [Eq. (73)].

We calculate the cap area using

$$\begin{aligned}
 A_{\text{cap}} &= \int \sqrt{1 + (\partial z / \partial x)^2 + (\partial z / \partial y)^2} dx dy \\
 &\approx \int \left\{ 1 + \frac{1}{2} [(\partial z / \partial x)^2 + (\partial z / \partial y)^2] \right\} dx dy \\
 &= A_{\text{base}} + \frac{1}{2} \int [(\partial z / \partial x)^2 + (\partial z / \partial y)^2] dx dy.
 \end{aligned} \tag{74}$$

Here the integrals go over the region defined by  $z(x, y) = R - h$ ,  $z(x, y)$  being given by Eq. (71). In the first step, we replaced the root by the Taylor expansion because the original integral cannot be evaluated analytically and in the second step we recognized that the first term in the curly brackets gives  $A_{\text{base}}$ ;  $\Delta A = A_{\text{cap}} - A_{\text{base}}$ .

After inserting  $z(x, y)$  from Eq. (71), we find that

$$A_{\text{cap}} \approx A_{\text{base}} + 2\pi \left( 1 - \frac{1}{m} \right) \csc \left( \frac{\pi}{m} \right) R^2 \left( \frac{\tilde{h}}{R} \right)^2. \tag{75}$$

In Fig. S9, this result is compared to the numerically obtained exact superball cap area.

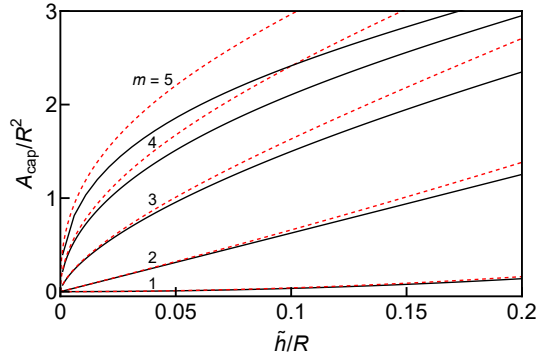

FIG. S9. Superball cap area vs.  $\tilde{h}/R$  for  $m = 1, 2, 3, 4$  and  $5$ : Exact results (black curves) vs. approximation based on the Monge representation [Eq. (75), dashed red curves].

The deformation free energy for the truncated superball shape is obtained by inserting Eqs. (56), (59), (72) (73) and (75) into Eq. (1) and minimizing it with respect to  $m$ .

## VI. TRUNCATED SPHEROPOLYHEDRON

The spheropolyhedron (also referred to as rounded or dilated polyhedron) is defined as a Minkowski sum of a polyhedron and a sphere and shown in Fig. S4b. These shapes are obtained by rounding the edges of a polyhedron such that their cross-section is circular; the shape of the thus obtained edges is cylindrical and the vertices are spherical. In spheropolyhedra, the mean curvature of the non-contact domain is non-uniform: At the rounded edges it is  $1/2R_{\text{edge}}$ , where  $R_{\text{edge}}$  is the radius of the curvature, whereas at the rounded vertices it is  $1/R_{\text{edge}}$ . The contact zones are polygons, generally of the same shape as the parent face; in truncated spheropolyhedra, the contact zones are rounded polygons as illustrated in Fig. S10.

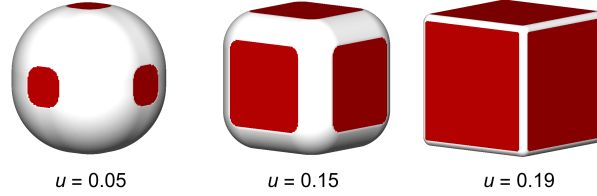

FIG. S10. Minimal-energy truncated spherocube shapes at  $\Psi = 10^{-3}$ ,  $\omega = 1$ , and  $u = 0.05, 0.15$ , and  $0.19$  like in Fig. S3. The  $u = 0.05$  and  $0.15$  shapes show how truncation, which increases with indentation up to  $u = 0.11$ , affects the contour of the contact zones at various indentations as indicated.

Spheropolyhedral shapes are parametrized by the relative radius of the edges

$$\mu = \frac{R_{\text{edge}}}{R_*}, \quad (76)$$

which equals 1 in the sphere and 0 in a polyhedron; there exists no sharp distinction between the partial, advanced, and complete faceting regimes.

### A. Truncated spherocube

The volume, contact area, and non-contact area of spheropolyhedra evidently depend on the shape of the parent polyhedron. Here we calculate them for a drop in the simple cubic (SC) lattice where the parent polyhedron is a cube, first for a non-truncated shape. The lattice constant  $a$  is given by Eq. (23) and the spherocube volume reads

$$\begin{aligned} V &= a^3 - 12(a - 2R_{\text{edge}}) \left( R_{\text{edge}}^2 - \frac{\pi}{4} R_{\text{edge}}^2 \right) - 8 \left( R_{\text{edge}}^3 - \frac{\pi}{6} R_{\text{edge}}^3 \right) \\ &= 8R_*^3 \left[ (1 - u)^3 - 3 \left( 1 - \frac{\pi}{4} \right) (1 - \mu - u) \mu^2 - \left( 1 - \frac{\pi}{6} \right) \mu^3 \right]. \end{aligned} \quad (77)$$

The area of the non-contact domain is

$$A_F = 4\pi R_{\text{edge}}^2 + 6\pi R_{\text{edge}}(a - 2R_{\text{edge}}) = 4\pi R_*^2 [\mu^2 + 3\mu(1 - \mu - u)] \quad (78)$$

and the area of the contact zones is

$$A_C = 6(a - 2R_{\text{edge}})^2 = 24R_*^2(1 - \mu - u)^2. \quad (79)$$

These expressions hold for all  $u$ .

The truncated spherocube is constructed by removing layers of identical thickness from the flat faces of the non-truncated spherocube. The thus created contact zones are squares with rounded corners rather than squares like in the non-truncated spherocube, the corner radius increasing with the degree of truncation (Fig. S10).

The cross-section of the truncated spherocube in the  $xz$  plane is shown in Fig. S11. In addition to  $\mu$  defined in Eq. (76), we parametrize this shape by

$$\eta = \frac{x_1}{R_*}. \quad (80)$$

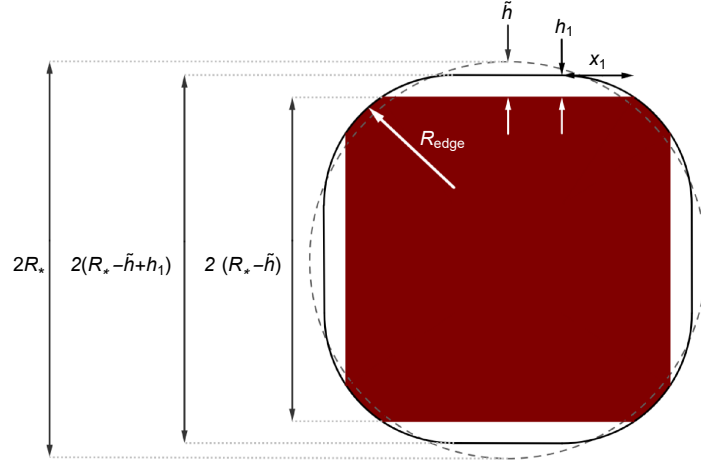

FIG. S11. Cross-section of the truncated spherocube cutting through the center across the  $xz$  plane, with the various distances of interest shown. The red domain is the non-truncated spherocube, the gray outline shows its truncated counterpart and the dashed line represents the isolated drop.

Here  $x_1$  is defined in Fig. S11; physically,  $2x_1$  is the difference of edge length of the square circumscribed around a face of the truncated spherocube and the edge length of a face of the parent non-truncated spherocube. If  $\eta = 0$  and  $\mu < 1$ , the shape is a spherocube whereas the limiting case  $\mu = 1$  and  $\eta > 0$  represents a truncated sphere. Note that

$$\frac{\eta}{\mu} \leq \frac{\sqrt{2}}{2}; \quad (81)$$

for  $\eta/\mu = \sqrt{2}/2$  the contact zones touch.

Apart from  $x_1$ , also important is the thickness of the shaved-off portions of the faces:

$$h_1 = R_{\text{edge}} - \sqrt{R_{\text{edge}}^2 - x_1^2} = R_* \mu \left[ 1 - \sqrt{1 - \eta^2/\mu^2} \right]. \quad (82)$$

In terms of the above quantities, the face-to-face distance in the spherocube prior to truncation reads

$$a = 2(R_* - h + h_1) = 2R_* \left\{ 1 - u + \mu \left[ 1 - \sqrt{1 - \eta^2/\mu^2} \right] \right\} \quad (83)$$

or in dimensionless form

$$\alpha = \frac{a}{R_*} = 2 \left\{ 1 - u + \mu \left[ 1 - \sqrt{1 - \eta^2/\mu^2} \right] \right\}, \quad (84)$$

where

$$u = \frac{h}{R_*} \quad (85)$$

is the dimensionless engineering indentation.

The volume of the truncated spherocube is obtained by subtracting the total volume of the three types of shaved-off bodies [specifically, 6 square layers of area  $(a - 2R_{\text{edge}}) \times (a - 2R_{\text{edge}})$  and thickness  $h_1$ ,  $6 \times 4 = 24$  cylindrical sections, and  $24 \times 1/4 = 6$  spherical caps] from the volume of the non-truncated spherocube given by Eq. (77):

$$\begin{aligned} V = & a^3 - 12(a - 2R_{\text{edge}}) \left( R_{\text{edge}}^2 - \frac{\pi}{4} R_{\text{edge}}^2 \right) - 8 \left( R_{\text{edge}}^3 - \frac{\pi}{6} R_{\text{edge}}^3 \right) \\ & - 6(a - 2R_{\text{edge}})^2 h_1 - 24V_{\text{cyl}} - 24V_{\text{sph}}. \end{aligned} \quad (86)$$

The volume of a single cylindrical section of length  $a - 2R_{\text{edge}}$ , radius  $R_{\text{edge}}$ , and width  $x_1$  is

$$\begin{aligned} V_{\text{cyl}} = & \frac{a - 2R_{\text{edge}}}{2} R_{\text{edge}}^2 \left[ \arcsin \left( \frac{x_1}{R_e} \right) - \frac{x_1}{R_e} \sqrt{1 - \left( \frac{x_1}{R_e} \right)^2} \right] \\ = & R_*^3 \frac{\alpha - 2\mu}{2} \mu^2 \left[ \arcsin(\eta/\mu) - (\eta/\mu) \sqrt{1 - \eta^2/\mu^2} \right]. \end{aligned} \quad (87)$$

(Limiting case: If  $x_1 = R_{\text{edge}}$ , we have  $V_{\text{cyl}} = (a - 2R_{\text{edge}}) \times \pi R_{\text{edge}}^2 / 4$ , that is a quarter of a cylinder. In reality,  $x_1 \leq \sqrt{2}R_{\text{edge}}/2$ .) The volume of the shaved-off spherical cap per vertex on a given face reads

$$\begin{aligned} V_{\text{sph}} &= \frac{\pi h_1^2}{4} \left( R_{\text{edge}} - \frac{h_1}{3} \right) = \frac{\pi}{12} \left( R_{\text{edge}} - \sqrt{R_{\text{edge}}^2 - x_1^2} \right)^2 \left( 2R_{\text{edge}} + \sqrt{R_{\text{edge}}^2 - x_1^2} \right) \\ &= \frac{\pi \mu^3 R_*^3}{12} \left( 1 - \sqrt{1 - \eta^2/\mu^2} \right)^2 \left( 2 + \sqrt{1 - \eta^2/\mu^2} \right). \end{aligned} \quad (88)$$

The area of the non-contact domain of the truncated spherocube is smaller than that of the non-truncated one [Eq. (78)] by  $24 \times (A_{\text{cyl}}^{\text{cap}} + A_{\text{sph}}^{\text{cap}})$ , where

$$A_{\text{cyl}}^{\text{cap}} = (a - 2R_{\text{edge}}) R_{\text{edge}} \arcsin(x_1/R_{\text{edge}}) = R_*^2 \mu (\alpha - 2\mu) \arcsin(\eta/\mu) \quad (89)$$

and

$$A_{\text{sph}}^{\text{cap}} = \frac{\pi R_{\text{edge}}^2}{2} \left( 1 - \sqrt{1 - x_1^2/R_{\text{edge}}^2} \right) = \frac{\pi R_*^2}{2} \mu^2 \left( 1 - \sqrt{1 - \eta^2/\mu^2} \right). \quad (90)$$

In turn, the contact area of the truncated spherocube is larger than that of the non-truncated one [Eq. (79)] by  $24 \times (A_{\text{cyl}}^{\text{base}} + A_{\text{sph}}^{\text{base}})$ , where

$$A_{\text{cyl}}^{\text{base}} = (a - 2R_{\text{edge}}) x_1 = R_*^2 (\alpha - 2\mu) \eta \quad (91)$$

and

$$A_{\text{sph}}^{\text{base}} = \frac{\pi x_1^2}{4} = R_*^2 \frac{\eta^2}{4}. \quad (92)$$

## B. Deformation free energy

The bulk term of the deformation free energy reads

$$\Delta F_{\text{bulk}} = \chi_T^{-1} \left[ \Delta V - V_0 \ln \left( 1 + \frac{\Delta V}{V_*} \right) \right], \quad (93)$$

where

$$\begin{aligned} \Delta V &= V - V_* \\ &= R_*^3 \left[ \alpha^3 - 12(\alpha - 2\mu) \mu^2 \left( 1 - \frac{\pi}{4} \right) - 8\mu^3 \left( 1 - \frac{\pi}{6} \right) - 6(\alpha - 2\mu)^2 \frac{h_1}{R_*} - 24 \frac{V_{\text{cyl}}}{R_*^3} - 26 \frac{V_{\text{cap}}}{R_*^3} - \frac{4\pi}{3} \right], \end{aligned} \quad (94)$$

Here  $\alpha, h_1, V_{\text{cyl}}$ , and  $V_{\text{cap}}$  are defined in Eqs. (84), (82), (86), and (88), respectively. The surface term of the deformation free energy is

$$\begin{aligned} \Delta F_{\text{surf}} &= 4\pi\gamma_F R_*^2 \left\{ \mu^2 \left[ 1 - 3 \left( 1 - \sqrt{1 - \eta^2/\mu^2} \right) \right] + \mu (\alpha - 2\mu) \left[ \frac{3}{2} - \frac{6}{\pi} \arcsin(\eta/\mu) \right] \right. \\ &\quad \left. + \frac{3}{2\pi} \omega \left[ (\alpha - 2\mu) (\alpha - 2\mu + 4\eta) + \pi \eta^2 \right] - 1 \right\}, \end{aligned} \quad (95)$$

where we used Eqs. (78), (79), (89), (90), (91), and (92). Thus the dimensionless deformation energy per contact (recall that in the SC lattice,  $z = 6$ ) is

$$\begin{aligned} \frac{\Delta F}{6\gamma_F R_0^2} &= \frac{4\pi}{9\Psi} \left[ \lambda_\Psi^3 \frac{\Delta V}{V_*} - \ln \left( 1 + \frac{\Delta V}{V_*} \right) \right] \\ &\quad + \frac{2\pi}{3} \lambda_\Psi^2 \left\{ \mu^2 \left[ 1 - 3 \left( 1 - \sqrt{1 - \eta^2/\mu^2} \right) \right] + \mu (\alpha - 2\mu) \left[ \frac{3}{2} - \frac{6}{\pi} \arcsin(\eta/\mu) \right] \right. \\ &\quad \left. + \frac{3}{2\pi} \omega \left[ (\alpha - 2\mu) (\alpha - 2\mu + 4\eta) + \pi \eta^2 \right] - 1 \right\}. \end{aligned} \quad (96)$$

This expression is minimized with respect to  $\mu$  and  $\eta$  so as to obtain the variational energy-minimizing state. The two constraints that need to be satisfied are: (i) the edges of the faces of the parent non-truncated spherocube should be finite, i.e.,  $a - 2R_{\text{edge}} \geq 0$ , which reduces to

$$\mu \leq \sqrt{(1-u)^2 + \eta^2} \quad (97)$$

(so that the limiting case where  $\mu = \sqrt{(1-u)^2 + \eta^2}$  corresponds to a truncated sphere), and (ii)  $V_{\text{cap}} > 0$ , which leads to  $\mu \geq \eta$ ; the latter condition is less restrictive than Eq. (81) and thus irrelevant.

In incompressible drops, i.e. for  $\Psi = 0$ ,  $\Delta V$  and thus the bulk term in Eq. (96) are zero and the constraint

$$V = \frac{4\pi R_*^3}{3}, \quad (98)$$

[where  $V$  is the spherocube volume given by Eq. (86)] is solved at a given  $u$  either for  $\mu$  or for  $\eta$ . The thus obtained  $\mu$  or  $\eta$  are then inserted into Eq. (96) and minimized.

In Fig. S12, the energy-minimizing  $\mu$  and  $\eta$  are plotted as functions of  $u$  for  $\Psi = 10^{-3}, 10^{-2}, \dots, 10^2$  and  $\omega = 1$ . As expected,  $\mu$  monotonically decreases with  $u$  whereas  $\eta$  is maximal at a finite  $u$  between about 0.1 and 0.2 depending on  $\Psi$ . At  $\Psi = 10^{-3}$ , both parameters drop to 0 at  $u \approx 0.2$ , indicating the onset of complete faceting. At the other  $\Psi$ 's shown, the decrease of  $\mu$  and  $\eta$  to 0 as  $u$  is increased is more gradual.

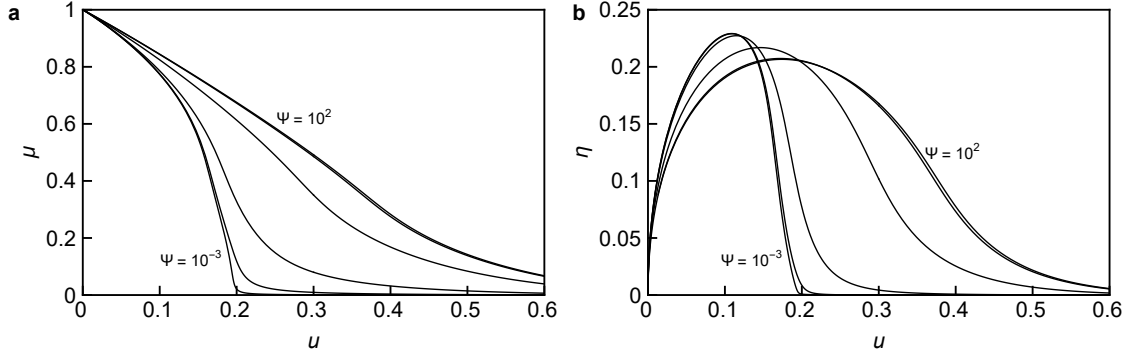

FIG. S12. Energy-minimizing parameters of the spherocube at  $\omega = 1$ :  $\mu$  (a) and  $\eta$  (b) vs.  $u$  for  $\Psi = 10^{-3}, 10^{-2}, \dots, 10^2$ , with all but the first and the last label omitted for clarity.

In Fig. S13, we compare the variational deformation energy for the non-truncated and the truncated spherocube model at  $\omega = 1$  and  $\Psi = 1, 10$ , and  $10^2$ . As expected, truncation lowers the variational energy, the effect being more prominent at small  $u$  where the magnitude of truncation is large as shown in Fig. S12. In Fig. S14, we plot the energy-minimizing  $\eta(u)$  for a few selected  $\omega \leq 1$ ; the results presented are for  $\Psi = 10^{-3}$ . This figure shows that truncation lowers the deformation energy only at  $1 \leq \omega \leq 1$  whereas at  $\omega \geq 1$  the energy-minimizing shapes are non-truncated. Also evident

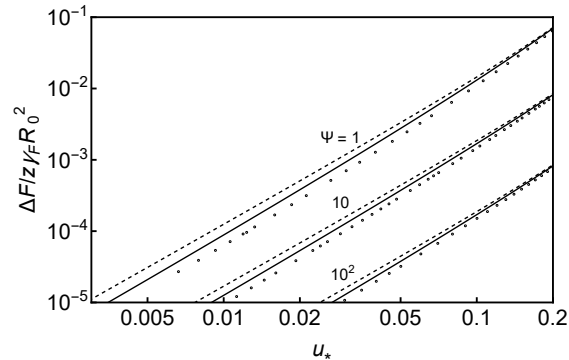

FIG. S13. Comparison of the deformation free energies of the non-truncated spherocube model (dashed lines) and the truncated spherocube model (solid lines) for  $\omega = 1$  and  $\Psi = 1, 10$  and  $100$ ; symbols show exact results.



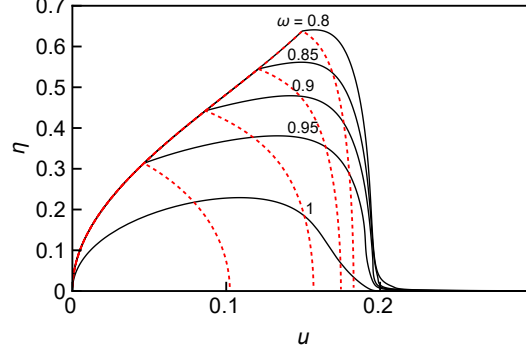

FIG. S14. Energy-minimizing  $\eta(u)$  at  $\Psi = 10^{-3}$  and  $\omega = 0.8, 0.85, 0.9, 0.95$ , and  $1$ . The dashed red lines at each  $\omega$  shows the constraint representing the truncated-sphere shape [Eq. (97)].

from this figure is the effect of the constraint in Eq. (97): For each  $\omega < 1$ , the energy-minimizing truncated spherocube shape reduces to a truncated sphere at indentations smaller than some  $u'$  that depends on  $\omega$  (NB: In this regime, the deformation free energy of the truncated superball is smaller still than that of the truncated sphere). The constraint in Eq. (97) can be rewritten as  $\eta \geq \sqrt{\mu^2 - (1-u)^2}$ . Since  $\mu$  decreases with increasing  $u$  beyond the point of departure from the constraint, the right-hand side of the inequality decreases with  $u$  and the bound on  $\eta$  tends to zero as seen in Fig. S14.

### C. Truncated spherotetrahedron

The construction of the truncated spherotetrahedron is completely analogous to that for the truncated sphere to but geometrically somewhat more involved; we only list the results. The volume of the truncated spherotetrahedron is

$$V = \frac{\sqrt{2}}{12} l'^3 + \sqrt{3} l'^2 (R_{\text{edge}} - h_1) + 3(\pi - \varphi) R_{\text{edge}}^2 l' - 12V_{\text{cyl}} + \frac{4\pi}{3} R_{\text{edge}}^3 - 12V_{\text{cap}} \quad (99)$$

where

$$l' = 2\sqrt{6}R_* \left[ 1 - u - \mu \sqrt{1 - \eta^2/\mu^2} \right]. \quad (100)$$

is the length of the edges,

$$V_{\text{cyl}} = \frac{R_{\text{edge}}^2}{2} \left[ \arcsin(\eta/\mu) - (\eta/\mu) \sqrt{1 - \eta^2/\mu^2} \right] l'. \quad (101)$$

is the volume of a single wedge-like portion of a rounded edge removed upon truncation, and

$$V_{\text{sph}} = \frac{\pi \mu^3 R_*^3}{9} \left( 1 - \sqrt{1 - \eta^2/\mu^2} \right)^2 \left( 2 + \sqrt{1 - \eta^2/\mu^2} \right). \quad (102)$$

is the volume of the part of the spherical cap removed upon truncation from a rounded vertex of the spherotetrahedron. Note that  $V_{\text{sph}}$  in the truncated spherotetrahedron corresponds to a  $\pi/3$  section of a spherical cap rather than to a  $\pi/4$  section of a spherical cap like in the truncated spherocube [Eq. (88)].

The area of the non-contact domain of the truncated spherotetrahedron reads

$$A_F = 4\pi R_{\text{edge}}^2 - 12A_{\text{sph}}^{\text{cap}} + 6(\pi - \varphi) R_{\text{edge}} l' - 12A_{\text{cyl}}^{\text{cap}}, \quad (103)$$

where

$$A_{\text{cyl}}^{\text{cap}} = (a - 2R_{\text{edge}}) R_{\text{edge}} \arcsin(x_1/R_{\text{edge}}) = R_*^2 \mu (\alpha - 2\mu) \arcsin(\eta/\mu) \quad (104)$$

is the cap area of a single wedge-like portion of a rounded edge removed upon truncation and

$$A_{\text{sph}}^{\text{cap}} = \frac{2\pi R_{\text{edge}}^2}{3} \left(1 - \sqrt{1 - x_1^2/R_{\text{edge}}^2}\right) = \frac{\pi R_*^2}{2} \mu^2 \left(1 - \sqrt{1 - \eta^2/\mu^2}\right). \quad (105)$$

is the cap area of the part of the spherical cap removed upon truncation from a rounded vertex. The contact area per truncated spherotetrahedron reads

$$A_C = 4 \left( \frac{\sqrt{3}}{4} l'^2 + 3x_1 l' + \pi x_1^2 \right) = 4 \left( \frac{\sqrt{3}}{4} l'^2 + 3 \frac{\eta}{R_*} l' + \pi \frac{\eta^2}{R_*^2} \right), \quad (106)$$

where  $x_1 l'$  represents the base area of a single portion of a rounded edge removed upon truncation  $A_{\text{cyl}}^{\text{base}}$  whereas  $\pi x_1^2/3$  is the base area of the part of the spherical cap removed from a rounded vertex  $A_{\text{sph}}^{\text{base}}$ .

Finally, the general form of the constraint in Eq. (81) is

$$\frac{\eta}{\mu} \leq \sqrt{1 - \sin^2\left(\frac{\varphi}{2}\right)} \quad (107)$$

where  $\varphi$  is the dihedral angle; in the tetrahedron,  $\varphi = \arccos(1/3)$  so that  $\eta/\mu \lesssim 0.816495$ . Using Eqs. (99)-(106), we calculate the deformation free energy  $\Delta F$  of a drop in the DC lattice. In Fig. S15a, we compare the results obtained using the truncated spherotetrahedron model to exact numerical results for  $\Psi = 10^{-3}$  and  $\omega = 0.8, 1$ , and  $1.2$ . Evidently the variational shape works rather well except in the attractive regime at  $u < 0.1$  and  $\omega < 1$ , where the best variational ansatz is the truncated tetrahedral superball (not shown for clarity). Figure S15b shows the variational and the exact  $\Delta F$  at  $\omega = 1$  and  $\Psi = 10^{-3}, 10^{-2}, \dots, 10^2$  in a log-log plot.

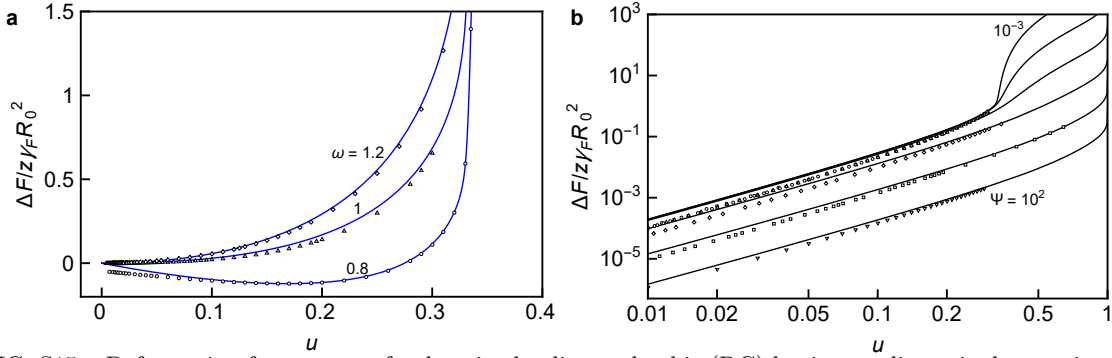

FIG. S15. Deformation free energy of a drop in the diamond cubic (DC) lattice vs. dimensionless engineering indentation. Panel (a) shows exact (symbols) and spherotetrahedron variational (solid lines) dimensionless  $\Delta F$  per contact for  $\Psi = 10^{-3}$  and  $\omega = 0.8, 1$ , and  $1.2$ . In panel (b), we plot  $\Delta F(u)$  for  $\omega = 1$  and  $\Psi = 10^{-3}, 10^{-2}, \dots, 10^2$  (top to bottom), again showing both exact (excluding  $\Psi = 10^{-1}$ ) and variational results (symbols and lines, respectively).

#### D. Simplified truncated spheropolyhedron

In the advanced faceting regime, the spheropolyhedral variational shape can be somewhat simplified by neglecting the rounded vertices and their contribution to volume, area, and energy. In this regime, the dimensionless radius of the rounded portions of the shape is much smaller than the resting radius (i.e.,  $\mu \ll 1$ ) and since the volumes of the rounded edges and vertices are proportional to  $\mu^2$  and  $\mu^3$ , respectively, the latter is subdominant and can be omitted. The same argument applies to the two terms in the area of the non-contact domain; the edge term scales as  $\mu$  and the vertex term scales as  $\mu^2$ . This approximation leads to somewhat simplified expressions for  $V, A_C, A_F$  and thus  $\Delta F$ , which offer a reasonable good description of both exact  $\Delta F$  and  $\Delta F$  obtained using the full unabbreviated spherocube shape as shown in Fig. S16.

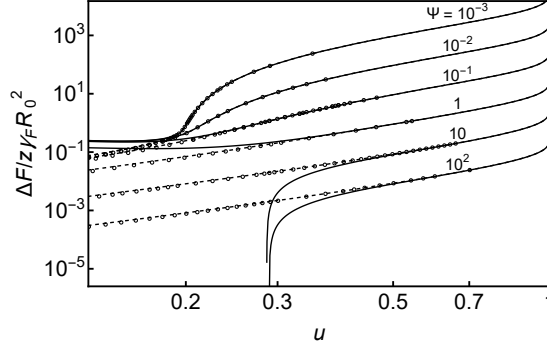

FIG. S16. Deformation free energy of drop in the SC lattice vs. indentation for  $\omega = 1$  and  $\Psi = 10^{-3}, 10^{-2}, \dots, 10^2$ : Exact results (symbols), full spherocube shape (dashes lines), and simplified spherocube shape (solid lines).

## VII. SCALING OF DEFORMATION FREE ENERGY

### A. Small-tension drops

In drops with  $\Psi \ll 1$  which are essentially incompressible, we observe two regimes where the deformation free energy depends on  $\Psi$  in some simple manner, one at small and the other at large indentations.

At small indentations, it suffices to see that for  $\Psi \ll 1$  the free energy given by Eq. (1) and conveniently rewritten as

$$\frac{F}{\gamma_F R_0^2} = \frac{8\pi}{3\Psi} \left( \frac{V}{V_0} - 1 - \ln \frac{V}{V_0} \right) + \frac{A_F}{R_0^2} + \omega \frac{A_C}{R_0^2}. \quad (108)$$

is dominated by the bulk term in that any deviation of  $V$  from the resting volume  $V_*$  imposed by indentation scales as  $(V/V_* - 1)/\Psi$  whereas the corresponding non-contact and contact surface terms scale as  $A_F/A_* - 1$  and  $A_C/A_*$ , respectively; here  $A_*$  is the area of the resting drop. As a result, the low-energy deformation mode involves area change at constant volume. In turn, the bulk term is absent from the deformation free energy, which is thus independent of  $\Psi$  as shown in Fig. 2b of the main text.

At large indentations where the drop is almost completely faceted, the non-contact area is much smaller than the contact area ( $A_F \ll A_C$ ) and can be neglected. In addition, in this regime the shape does not depend on indentation so that

$$A_C(\omega, u) \propto V(\omega, u)^{2/3}, \quad (109)$$

where the omitted numerical coefficient depends on the shape; in a cube, its value is 6. As  $u$  is increased, both  $V$  and  $A_C$  decrease and eventually vanish at  $u = 0$ . This makes the surface energy of the contact zones much smaller than the bulk free energy, which diverges because of the ideal-gas term. As a result, the contact surface energy can be dropped too. Finally, we note that in the complete faceting regime the deformation free energy is much larger than the resting energy  $F_*(\Psi)$  so that  $\Delta F(u) = F(u) - F_* \approx F(u)$ .

The volume of a completely faceted drop is of the form

$$V = \beta V_*(1 - u)^3, \quad (110)$$

where  $\beta$  depends on drop shape; in a cube,  $\beta = 6/\pi$ . Thus in the complete faceting regime, the deformation free energy reduces to

$$\begin{aligned} \frac{\Delta F(\Psi \ll 1, u)}{\gamma_F R_0^2} &\approx \frac{8\pi}{3\Psi} \left( \frac{V}{V_0} - 1 - \ln \frac{V}{V_0} \right) \\ &= \frac{8\pi}{3\Psi} [\beta(1 - u)^3 - 1 - \ln(\beta(1 - u)^3)]. \end{aligned} \quad (111)$$

In the last step, we neglected the subdominant terms in  $\Psi$  for clarity; these terms arise from the deviation of the ratio  $R_*/R_0 = \lambda_\Psi \approx 1 - \Psi/3$  [Eq. (8)] from unity at  $\Psi \ll 1$ . Together with Eq. (115) derived below, Eq. (111) shows that the scaling  $\Delta F \propto \Psi^{-1}$  applies at all  $\Psi$  provided that  $u$  is large enough. This is seen in Fig. 2b of the main text.

### B. Large-tension drops

In the large-tension drops where  $\Psi \gg 1$ , the bulk free energy [Eq. (1)] is dominated by the repulsive, ideal-gas term  $\chi_T^{-1} V_0 \ln(V/V_0)$ . If we omit the subdominant term  $\chi_T^{-1}(V - V_0)$  from the bulk free energy, we find that

$$\frac{F(\Psi \gg 1)}{\gamma_F R_0^2} \approx -\frac{8\pi}{3\Psi} \ln \frac{V}{V_0} + \frac{A_F}{R_0^2} + \omega \frac{A_C}{R_0^2}. \quad (112)$$

In this regime, the resting radius of an isolated spherical drop is given by Eq. (9):  $\lambda_\Psi \approx 1/\sqrt{\Psi}$ .

We now assume that at any  $\Psi \gg 1$ , drop shape depends on indentation  $u$  and on the tension ratio  $\omega$  but not on  $\Psi$ , that is

$$\begin{aligned} V(\omega, u) &= V_* f_V(\omega, u), \\ A_F(\omega, u) &= A_* f_F(\omega, u), \\ A_C(\omega, u) &= A_* f_C(\omega, u). \end{aligned} \quad (113)$$

Here  $V_* = 4\pi R_*^3/3$ ,  $A_* = 4\pi R_*^2$ , and  $f_V, f_F$ , and  $f_C$  are some dimensionless functions that depend on  $\omega$  and  $u$  but not on  $\Psi$ ; in the resting drop (i.e., at  $u = 0$ ),  $f_V = f_F = 1$  and  $f_C = 0$ . Figure S17 shows these functions obtained using the truncated spherocube model at  $\Psi = 1, 10$  and  $10^2$  (blue, red, and black line, respectively) and  $\omega = 1$ .

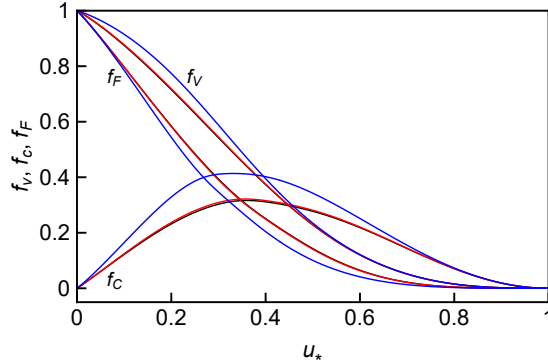

FIG. S17. Functions  $f_V, f_F$ , and  $f_C$  obtained using truncated spherocube variational shapes at  $\Psi = 1, 10$ , and  $10^2$  (blue, red, and black line, respectively) and  $\omega = 1$ .

Upon inserting the ansätze in Eq. (113) and Eq. (9) into Eq. (112), we obtain

$$\frac{F(\Psi \gg 1)}{\gamma_F R_0^2} \approx \frac{4\pi}{\Psi} \left( -\frac{2}{3} \ln \frac{f_V}{\Psi^{3/2}} + f_F + \omega f_C \right). \quad (114)$$

As the energy of the resting drop is  $F_*(\Psi \gg 1)/\gamma_F R_0^2 \approx (4\pi/\Psi) (\ln \Psi + 1)$ , the deformation free energy  $\Delta F = F - F_*$  reduces to

$$\frac{\Delta F(\Psi \gg 1)}{\gamma_F R_0^2} \approx \frac{4\pi}{\Psi} \left( -\frac{2}{3} \ln f_V + f_F + \omega f_C - 1 \right). \quad (115)$$

This scaling with  $\Psi$  is seen in both exact and variational results in Fig. 2b of the main text, and it applies at all indentations  $u$ .

### VIII. POWER LAWS OF LIQUID-DROP MODEL

For  $\omega \geq 1$  where the drop-drop interaction is repulsive at all indentations, the exact deformation free energy can be approximated by a suitable power law at small enough indentations. For the SC lattice, the best-fit exponents obtained by fitting  $\Delta F$  at  $u < 0.1$  by  $u^\alpha$  are listed in Table S1 for various  $\Psi$  and  $\omega = 1$  and 1.2. We note that the limiting values of the exponent at  $\Psi \ll 1$  and  $\Psi \gg 1$  are well-defined.

TABLE S1. Best-fit power-law exponents  $\alpha$  for  $\Psi = 10^{-3}, 10^{-2}, \dots, 10^2$  and for  $\omega = 1$  and 1.2.

|                        | $\Psi$    |           |           |      |        |        |
|------------------------|-----------|-----------|-----------|------|--------|--------|
|                        | $10^{-3}$ | $10^{-2}$ | $10^{-1}$ | 1    | $10^1$ | $10^2$ |
| $\alpha(\omega = 1)$   | 2.58      | 2.56      | 2.55      | 2.37 | 2.28   | 2.24   |
| $\alpha(\omega = 1.2)$ | 2.20      | 2.21      | 2.14      | 2.03 | 1.87   | 1.88   |

The functional form of  $\alpha(\Psi)$  can be approximated by

$$\alpha(\Psi) = \frac{\alpha_0 + \alpha_\infty \Psi}{1 + \Psi}, \quad (116)$$

where  $\alpha_0$  and  $\alpha_\infty$  are the values of the exponent at  $\Psi = 0$  and  $\infty$ , respectively, which both depend on  $\omega$ . We also find that at  $\omega = 1$  and 1.2, the deformation free energy for  $\Psi \geq 1$  per contact goes roughly as

$$\frac{\Delta F}{z\gamma_F R_0^2} \approx \frac{3}{\Psi} u^\alpha. \quad (117)$$

- 
- [1] K. A. Brakke, Exp. Math. **1**, 141 (1992).
  - [2] A.-K. Doukas, C. N. Likos, and P. Ziherl, Soft Matter **14**, 3063 (2018).
  - [3] Á. González García, J. Opdam, and R. Tuinier, Eur. Phys. J. E **41**, 63 (2018).
  - [4] S. I. R. Castillo, D. M. E. Thies-Weesie, and A. P. Philipse, Phys. Rev. E **91**, 022311 (2015).
